# Supplementary material for: Supply the Global, Supervise the Local: Combining Representation Conditioning and Alignment in Diffusion Transformers
Source: arXiv:2611.29138 source file (2026-11-22)
Supplement: Supplementary file 1 [file appendix_labels.tex]

\makeatletter
\begingroup
\appendix
\def\gclab#1#2#3{\setcounter{#1}{#2}\refstepcounter{#1}\global\let\@currentHref\@empty\label{#3}}
\gclab{section}{0}{sec:supp_related}
\setcounter{section}{2}\gclab{subsection}{0}{sec:proof_shares}
\setcounter{section}{2}\gclab{subsection}{2}{sec:visualization_protocol}
\gclab{section}{2}{sec:supp_probes}
\setcounter{section}{4}\gclab{subsection}{0}{sec:supp_input}
\setcounter{section}{4}\gclab{subsection}{1}{sec:atten-exp-settings}
\gclab{figure}{6}{fig:mech_usage}
\gclab{section}{4}{sec:supp_full}
\setcounter{section}{5}\gclab{subsection}{0}{sec:supp_variants}
\gclab{table}{7}{tab:supp_interaction}
\setcounter{section}{5}\gclab{subsection}{2}{sec:supp_specificity}
\setcounter{section}{5}\gclab{subsection}{3}{sec:supp_placement}
\setcounter{section}{5}\gclab{subsection}{4}{sec:supp_weight}
\gclab{section}{5}{sec:supp_impl}
\setcounter{section}{6}\gclab{subsection}{1}{sec:implementation-gc-repa}
\gclab{figure}{10}{fig:supp_probe_t}
\gclab{algorithm}{0}{alg:train}
\setcounter{section}{6}\gclab{subsection}{1}{sec:supp_cfg}
\setcounter{section}{7}\gclab{subsection}{0}{sec:supp_sources}
\setcounter{section}{7}\gclab{subsection}{1}{sec:supp_mem}
\setcounter{section}{7}\gclab{subsection}{2}{sec:alt_tokens}
\setcounter{section}{8}\gclab{subsection}{0}{sec:supp_t2i}
\gclab{table}{13}{tab:supp_t2i}
\setcounter{section}{8}\gclab{subsection}{1}{sec:supp_denoise}
\setcounter{section}{8}\gclab{subsection}{2}{sec:supp_grad}
\setcounter{section}{8}\gclab{subsection}{3}{sec:supp_compute}
\setcounter{section}{8}\gclab{subsection}{4}{sec:supp_encoders}
\gclab{section}{8}{sec:supp_samples}
\gclab{figure}{18}{fig:supp_tokgrid}
\endgroup
\makeatother
